# Supplementary material for: In-N-Out: Faithful 3D GAN Inversion with Volumetric Decomposition for Face Editing
Source: arXiv:2302.04871 source file (2024-04-14)
Supplement: Supplementary file 2 [file supp_content_arxiv.tex]

\section{Implementation details}
This section discusses further details not included in the main paper due to the page limit.

\subsection{In-distribution inversion}
We further present the details in Section {\color{blue}4.1} in the main paper. 

\topic{Latent code initialization.} 
Instead of initializing the latent codes $[w_1, \cdots, w_N], w_t \in \mathbb{R}^{14 \times 512}$ using an average latent code, we propose to use the nearest neighbor (NN) approach for the initialization. 
We show our approach in Algorithm~\ref{alg:nn_init}.

\input{algorithms/NN_initial.tex}

\topic{Optimization.} 
As mentioned in Section {\color{blue}4.1} in our main paper, we use a residual form to represent the latent code of each frame.
\begin{equation}
    w_t = w^{cano} + a w^{res}_t \,,
\end{equation}
where $w^{cano}$ is the canonical latent code, and $w^{res}_t$ is the residual. In practice, we use $a = 0.7$.

During the optimization, we first sample $K=16$ frames from the entire video.
For the subset optimization, we use $M_1 = 200$; to upscale the result to the whole video, we use $M_2 = 20$. 
The optimizer is Adam~\cite{kingma2014adam}. 
The learning rate is $5\times10^{-3}$.
To initialize the latent codes, we randomly sample $n=500$ latent codes.

\subsection{Out-of-domain inversion}
We further explain the details in Section {\color{blue}4.2} in the main paper. 

\topic{Tri-plane.}
We use the Tri-plane representation from EG3D~\cite{chan2022efficient}. 
For the out-of-distribution (OOD) object, we use tri-plane $\mathbf{T}^{O} \in \mathbb{R}^{256\times256\times32\times3}$ as its 3D representation. 
$\mathbf{T}^{O}$ is initialized from a standard normal distribution. 
Given a 3D position $\mathbf{x} \in \mathbb{R}^{3}$, we project it onto each of the plane and retrieve the corresponding feature vectors $F_{xy}, F_{yz}, F_{xz}$ through a bilinear interpolation. 
Then three feature vectors are aggregated via summation. 

\topic{Per-frame latent code $\mathbf{\phi}_t$.} To encode the OOD object across different frames, we use a time-varying latent code $\mathbf{\phi}_t \in \mathbb{R}^{32}$ for each frame. We draw $\mathbf{\phi}_t \sim \mathcal{N}(\mathbf{0}, \mathbf{I})$. 
$\mathbf{\phi}_t$ is optimized together with other variables in Section {\color{blue}4.2}.

\topic{Decoder.} For the out-of-distribution inversion, we use a two-layer Multi-Layer Perceptron (MLP) as the decoder to predict the pointwise color $\mathbf{c} \in \mathbb{R}^3$, density $\sigma \in \mathbb{R}$, and blending weight $b \in \mathbb{R}$ for the later composite rendering.
\begin{equation}
    (\mathbf{c}^O, \sigma^O, b) = D^O(\mathbf{T}^O(t_k), \mathbf{\phi}_t; \theta_{D^O}) \,.
\end{equation}

\topic{Optimization.} During the optimization, we use the loss function Eqn. {\color{blue}7} in the main paper. 

\subsection{Post-processing}\label{sec:postprocess}
We can put the aligned frames back into the original input video as an optional step. 
We use a face parsing algorithm~\cite{yu2021bisenet} to get the face segmentation 
and paste the face back to the input frame with a Gaussian Blur to smooth the boundary.
Finally, we paste the cropped, aligned frame into the full-resolution input video.

% \subsection{Composite volume rendering}
% \topic{Optimization.}

\subsection{Semi-supervised framework}
\begin{figure*}
\begin{center}
\centering
\includegraphics[trim=0 0 0 0, clip,width=0.9\textwidth]{images/method_overview_semi_sup.pdf}

\caption{
\textbf{Overview of our semi-supervised method.} 
Given a monocular portrait video, we use two radiance fields to represent 
(a) \textit{in-distribution} face, and (b) \textit{out-of-distribution (OOD)} item. 
(a) \textbf{In-distribution reconstruction} is the \textit{GAN inversion} for the in-distribution face. 
We apply GAN inversion to each frame, but exclude the pixels within the OOD mask $M_t$. 
We perform GAN inversion by using pre-trained EG3D model $G$, where the pre-trained tri-plane generator and tri-plane decoder $D^I$ are kept frozen. 
% The inversion is conducted based on a pre-trained EG3D model $G$, in which the tri-plane generator and tri-plane decoder $D^I$ are both pre-trained and frozen. 
(b) For \textbf{out-of-distribution} elements, we propose to model them with a separate radiance field described by an additional tri-plane $\mathbf{T}^O$. 
During the training process, we optimize the tri-plane $\mathbf{T}^O$, a per-frame latent code $\mathbf{\phi}_t$, and a new decoder $D^O$ with a masked reconstruction loss.
The decoder takes as input tri-plane features $\mathbf{T}^O$ and $\mathbf{\phi}_t$ and outputs color $\mathbf{c}^O$, density $\sigma^O$, and blending weight $b$. 
(c) \textbf{Composite Rendering} compose the \textit{in-distribution} and \textit{out-of-distribution} radiance fields together by using a composite rendering scheme. 
(d) Finally, we finetune the \textbf{Super Resolution} module in $G$ to achieve a better output in the high resolution.
After training, we can perform various semantic edits and free-view rendering, while preserving the face identity and the OOD components. 
}
\label{fig:method_overview_semi_sup}
\end{center}
\vspace{-5mm}
\end{figure*}

Our framework can be modified to work with user-given segmentation masks like previous works on NeRFs~\cite{gao2021dynamic,yang2021learning}. 
% With \emph{one} manually labeled OOD mask, we propagate this mask to other frames using an off-the-shelf tracking algorithm Xmem~\cite{cheng2022xmem}. 
Given an aligned, monocular face video $\mathbf{V}=[\mathbf{I}_1,\cdots, \mathbf{I}_t, \cdots, \mathbf{I}_N]$ with $N$ frames, 
and binary masks $[\mathbf{M}_1, \cdots, \mathbf{M}_t, \cdots, \mathbf{M}_N]$ of the out-of-distribution (OOD) content for each frame, 
we aim to reconstruct the video with EG3D inversion and perform face editing. 
For each video, we label the \emph{first frame} for $\mathbf{M}_1$, and use an off-the-shelf tracking algorithm~\cite{cheng2022xmem} to propagate it to obtain other masks $\mathbf{M}$'s.
We show the overview of our semi-supervised framework in Figure~\ref{fig:method_overview_semi_sup}.

\topic{Diffrence.} The main difference between our unsupervised framework (shown in our main paper) and semi-supervised framework is that we introduce two additional reconstruction loss functions for the in-distribution radiance field and the out-of-distribution radiance field, respectively. 
This is because we can use 2D masks to segment the in-distribution and out-of-distribution parts. 

\topic{In-distribution radiance field.} The optimization goal for the in-distribution radiance field is
\begin{equation}\label{eqn:goal_id}
    % \scriptsize
        \begin{split}
        % w^{*}_t, p^{*}_t & = \argmin_{w_t, p_t} \mathcal{L}^{I}_t  = 
        w^{*}_t &= \argmin_{w_t} \mathcal{L}^{I}_t  = 
        \argmin_{w_t} \frac{1}{||\mathbf{m}_t||_1}||\mathbf{m}_t \odot (\mathbf{x} - \mathbf{\hat{x}})||^2_2 \\ 
        &+ \mathcal{L}_{\mathrm{mLPIPS}}(\mathbf{x}, \mathbf{\hat{x}}, \mathbf{m}_t)
        + \lambda_{\Delta} \mathcal{L}_{\Delta} (w_t)  \,,
    \end{split}
\end{equation}
where $w_t$ is the latent code at time $t$, $\mathbf{x}$ is the input frame $\mathbf{I}_t$, $\mathbf{\hat{x}}$ is generation output $G(w_t, p_t)$, $\mathbf{m_t}=1-\mathbf{M}_t$, and $\mathcal{L}_{\mathrm{mLPIPS}}(x, \hat{x}, \mathbf{m})$ is the masked version of LPIPS loss~\cite{zhang2018perceptual}. 
Here, $p_t$ is the camera parameters estimated by~\cite{deng2019accurate}.
The masked LPIPS only considers features inside the mask $\mathbf{m}$.  
$\mathcal{L}_{\Delta}(w)= \sum^{13}_{i=1}||\Delta_i||^2_2$ is a regularization loss adopted from~\cite{tov2021designing}, used to constrain the variation among style vectors in $w$
given a latent code $w = (w_0, w_0 + \Delta_1, ..., w_0 + \Delta_{13}) \in \mathbb{R}^{14\times512}$. 
By minimizing the variation, we push $w \in \mathcal{W}^{+}$ to be closer to $\mathcal{W}$ space, which has better editability.

We do not directly optimize for all the latent codes at once to speed up the optimization.
Instead, we first sample a subset of frames with corresponding initial latent codes from the video.
We optimize for these sampled latent codes, get the canonical latent code,
and then upscale it to all the frames for a few epochs. 
We find this can speed up the optimization and keep good reconstruction quality for the whole video.
% We show our optimization pseudocode in Algorithm~\ref{alg:id_invert}.
% \input{algorithms/ID_inversion.tex}

We first sample $K=16$ frames from the whole video during our optimization.
For the subset optimization, we use $M_1 = 200$; to upscale the result to the whole video, we use $M_2 = 20$. 
The optimizer is Adam~\cite{kingma2014adam}. 
The learning rate is $5\times10^{-3}$.
To initialize the latent codes, we randomly sample $n=500$ latent codes.

\topic{Out-of-distribution radiance field.} The optimization objective is:
\begin{equation}\label{eqn:goal_ood}
    % \scriptsize
    \begin{split}
        & \mathbf{T}^{O*}, \theta^{*}_{D^O}, \mathbf{\phi}^{*}_t  = \argmin_{\mathbf{T}^O, \theta_{D^O}, \mathbf{\phi}_t} \mathcal{L}^{O}_t \\
        & = \argmin_{\mathbf{T}^O, \theta_{D^O}, \mathbf{\phi}_t} \sum_{ij} ||(\mathbf{C}^O_t(\mathbf{r}_{ij}) - \mathbf{C}^{GT}(\mathbf{r}_{ij})) \cdot \mathbf{M}_t(\mathbf{r}_{ij})||^2_2   \,,
    \end{split}
\end{equation} 
where $\mathbf{T}^O(t_k) \in \mathbb{R}^{32}$ is the aggregated features obtained by projecting 3D coordinate $t_k$ onto each of the three feature planes via bilinear interpolation, then aggregated via summation~\cite{chan2022efficient}.
The decoder $D^O$ is an MLP with weights of $\theta_{D^O}$. $\mathbf{C}^{GT}(\mathbf{r}_{ij})$ is the ground-truth color at pixel $(i,j)$.

\topic{Composite rendering.} The goal is 
\begin{equation}\label{eqn:goal_comp}
    % \scriptsize
    \begin{split}
        & \mathbf{T}^{O*}, \theta^{*}_{D^O}, \mathbf{\phi}^{*}_t = \argmin_{\mathbf{T}^O, \theta_{D^O}, \mathbf{\phi}_t} \mathcal{L}^C_t   \\
        &= \argmin_{\mathbf{T}^O, \theta_{D^O}, \mathbf{\phi}_t} \sum_{ij}||C^C(\mathbf{r}_{ij}) - C^{GT}(\mathbf{r}_{ij})||^2_2   \\
        &+ \lambda_{b}\mathcal{L}_b(\mathbf{r}_{ij}) + \sum_{\mathbf{M}_t(ij) \neq 1}\lambda_{spar}\mathcal{L}_{spar} + \mathcal{L}_{LPIPS}(\mathbf{I}^C_{LR}, \mathbf{I}_{LR})
        \,,
    \end{split}
\end{equation}
where $\mathcal{L}_{LPIPS}$ is LPIPS loss~\cite{zhang2018perceptual}, $\mathbf{I}^C_{LR}$ is the composite rendered image at low resolution ($128\times128$), $\mathbf{I}_{LR}$ is the ground truth image also at $128\times128$.
$\mathcal{L}_{spar}$ is a sparsity loss used to suppress the blending weights for the OOD pixels outside the mask. 
We use this regularization in case the OOD radiance field dominates, which makes the editing trivial, 
since we rely on the in-distribution part for the editing. 
\begin{equation}\label{eqn:spar_loss}
    \mathcal{L}_{spar}(\mathbf{r}) = \sum^K_{k=1} \mathcal{L}_1(b(t_k)) \,, 
\end{equation}
weight regularizer $\mathcal{L}_b$ is adopted from~\cite{wu2022d}, used to penalize the blending weight $b$ if it is not closer to 0 or 1:
\begin{equation}\label{eqn:blendw_loss}
    \mathcal{L}_b(\mathbf{r}) = \sum^K_{k=1} H_b(b(t_k)) \,,
\end{equation}
where $H_b(x) = -(x\log(x) + (1 - x)\log(x))$ is binary entropy.
The reason behind Eqn.~\ref{eqn:blendw_loss} is that objects cannot co-occupy \emph{the same spatial location}.
The entropy loss facilitates a cleaner decomposition to be either an in-distribution object (\ie $b \rightarrow 0$) or an out-of-distribution object (\ie $b \rightarrow 1$).

In practice, we optimize for Eqn.~\ref{eqn:goal_id} only. 
We then jointly optimize for Eqn.~\ref{eqn:goal_ood} and Eqn.~\ref{eqn:goal_comp}. 

\section{Additional results for Semi-Supervised method}
We compare our unsupervised framework and our semi-supervised framework. 

\topic{Hyperparameters.} We use the Adam optimizer~\cite{kingma2014adam} for all the experiments. 
For in-distribution inversion, we optimize for 200 epochs with a learning rate of $1\times10^{-3}$, the weight of latent variation loss $\lambda_{\Delta}$ = $1\times10^{-3}$.
For the out-of-distribution and composite rendering, we run the optimization for 200 to 300 epochs depending on the video length with a learning rate of $5\times10^{-3}$, the weight of blending weight regularizer $\lambda_b=1$, and the weight of sparsity loss $\lambda_{spar}=3$. 
For the SR module, we fine-tune the module for 100 epochs with a learning rate of $1\times10^{-3}$.

\topic{Reconstruction.} Compared to the semi-supervised method, our unsupervised method performs slightly worse. This is because the semi-supervised method works with segmentation masks, which is easier to split a frame into in-distribution and out-of-distribution parts. 

\begin{table}[h!]
  \centering
  \tiny	
  \caption{Quantitative comparison for reconstruction quality.}
    \begin{tabular}{lrrrrr}
    \toprule
    Metrics & \multicolumn{1}{l}{LPIPS$\downarrow$} & \multicolumn{1}{l}{$\mathcal{L}_2$$\downarrow$} & SSIM$\uparrow$ & \multicolumn{1}{l}{PSNR$\uparrow$} & \multicolumn{1}{l}{ID similarity$\uparrow$}  \\
    \midrule
    Ours (semi-supervised) & \textbf{0.1981}  &  \textbf{0.0150}  &   \textbf{0.7722}    &   \textbf{19.6985}    &   \textbf{0.9831}            \\
    Ours (unsupervised)   & \underline{0.2237}  & \underline{0.0339}  &   \underline{0.7052}    &   \underline{16.0287}    &  \underline{0.9758} \\
    \midrule
    PTI~\cite{roich2022pivotal}    & 0.3144   & 0.0504  &   0.6320    &  13.4483     &     0.9658       \\
    IDE-3D~\cite{sun2022ide}  &  0.4999  & 0.1172  &   0.4512    &   9.5852    &    0.8251         \\
    $\mathcal{W^{+}}$  & 0.3380  & 0.0383   &    0.6557   &    14.7486 &   0.9154     \\
    $\mathcal{W}$ & 0.4030  & 0.0618   &   0.5787    &      12.4769 & 0.8652       \\
    \bottomrule
    \end{tabular}%
  \label{tab:quant_inv}%
  \vspace{-3mm}
\end{table}%

\topic{Editing.} We report the evaluation of editing in Table~\ref{tab:quant_edit}. Similar to the reconstruction, the semi-supervised method preserves better editability. This is because, with masks to separate the in-distribution and out-of-distribution radiance fields, we make the in-distribution part (generated by the latent code) lie closer to the latent space of the pre-trained EG3D. This enables better editability.

\begin{table}[h!]
  \centering
  \tiny
  \caption{Quantitative comparison for identity preservation after editing. Higher numbers indicate better identity preservation.}
    \begin{tabular}{lrrrrr}
    \toprule
          & \multicolumn{1}{l}{``eyeglasses''} & \multicolumn{1}{l}{``surprised''} & \multicolumn{1}{l}{``younger''} & \multicolumn{1}{l}{``smile''} & \multicolumn{1}{l}{``Elsa''} \\
      \midrule
    Ours (semi-supervised)   &   \textbf{0.9368}    &   \textbf{0.9816}    & \textbf{0.9457} &   \textbf{0.9556}    & {0.8610} \\
    Ours (unsupervised)   & \underline{0.9158} & \underline{0.9360} & \underline{0.9347}  & {0.9094}     & \underline{0.8927}  \\
     \midrule 
    PTI  &   0.9049    &   0.9357    &  0.9319    &    \underline{0.9336}   & 0.7945  \\
    IDE-3D  &   0.8767    &   0.9481    &  0.8551     &   0.8662     &  0.7871 \\
    $\mathcal{W^{+}}$  &  0.8971     &  0.9249     &   0.9290    & 0.9170 & 0.7968  \\
    $\mathcal{W} $  &   0.8793    &  0.9537     &  0.9068      &    0.9208   & 0.8113  \\
    \bottomrule
    \end{tabular}%
  \label{tab:quant_edit}%
  % \vspace{-5mm}
\end{table}%

% \topic{Visual results.} Please refer to our \href{run:./pages/UnSupervised_vs_SemiSupervised.html}{Unsupervised v.s. Semi-Supervised page} for more visual results. 

\topic{Speed.} We also report the speed of different approaches in Table~\ref{tab:comp_speed}. The semi-supervised method is slower than the unsupervised method due to an additional loss function (Eqn.~\ref{eqn:goal_ood}). 

\begin{table}[h!]
    \centering
    \footnotesize	
    \caption{Speed for different baselines on 200 frames.}
    \begin{tabular}{cccc}
    \toprule
          PTI~\cite{roich2022pivotal}  &  IDE-3D~\cite{sun2022ide}  & Ours (unsupervised)  & Ours (semi-supervised) \\
    \midrule
          2.18h     &     95s     &  3.17h  &  3.54h \\
    \bottomrule
    \end{tabular}
    \label{tab:comp_speed}
\end{table}

\topic{Conclusion.} Compared to the semi-supervised method, our proposed unsupervised method
\begin{itemize}[noitemsep,topsep=0pt, leftmargin=*]
    \item works automatically without humans in the loop,
    \item converges faster than the semi-supervised method,
    \item but performs slightly worse than the semi-supervised method.
\end{itemize}
This enables different application scenarios given our proposed framework. If we have the segmentation masks, either from off-the-shelf algorithms or manual labels, then we can use them to achieve better performance. 
However, if we pursue a fully automatic approach, then our unsupervised framework can be used.
